# Supplementary material for: UKTA: Unified Korean Text Analyzer
Source: arXiv:2502.09648 source file (2025-02-11)
Supplement: Supplementary file 1 [file 00_Appendix.tex]

%===================================================================
\begin{table*}[th!]
\centering
\caption{\textbf{Impact of error propagation from Korean morpheme analysis on feature analysis results.} \textnormal{The \ash{red color} indicates incorrect results in morphological and selected feature (\textbf{NDW}, \textbf{TTR}, \textbf{CTTR}, \textbf{NNL\_Den}, \textbf{EFL\_Den}) analysis compared to the ground truth (black color). Romanized expressions in Korean are denoted using \textit{italic}, and $/⟨TAG⟩$ represents the part-of-speech (POS) tag in morpheme analysis. The POS tags and feature descriptions are provided in Tables \ash{[todo]} and \ash{[todo]}, respectively.}}
%Even eojeols having the same sequences of characters can diverge in meaning depending on the combination of morphemes. Roman expressions in Korean are denoted using \textit{italic}. /$\langle$TAG$\rangle$ in morpheme represents the POS tag.}
\resizebox{1\textwidth}{!}{%
% \begin{threeparttable}
\setlength\tabcolsep{8pt}
\begin{tabular}{cccccccccc}
    \toprule
    % \textbf{Input text} & \multicolumn{10}{c}{\makecell*{\textbf{\underline{나는}} 하늘을 \textbf{\underline{나는}} 나비를 봤다  \\ \textit{\textbf{\underline{Naneun}} haneureul \textbf{\underline{naneun}} nabireul bwatda} \\ (I saw a butterfly flying in the sky)}} \\
    %\midrule
    \multicolumn{5}{c}{\textbf{Input text}} & \multicolumn{5}{c}{\textbf{Wordpiece analysis}} \\
    \cmidrule(r){1-5} \cmidrule(l){6-10}
     \multicolumn{5}{c}{\makecell*{\textbf{\underline{나는}} 하늘을 \textbf{\underline{나는}} 나비를 봤다  \\ \textit{\textbf{\underline{Naneun}} haneureul \textbf{\underline{naneun}} nabireul bwatda} \\ (I saw a butterfly flying in the sky)}} & \makecell*{나는 \\ \textit{Naneun} \\ (I)} & \makecell*{하늘을 \\ \textit{haneureul} \\ (in the sky)} & \makecell*{나는 \\ \textit{Naneun} \\ (flying)} & \makecell*{나비를 \\ \textit{nabireul} \\ (a butterfly)} &\makecell*{봤다 \\ \textit{bwatda} \\ (saw)} \\
    \midrule
    \multicolumn{5}{c}{}&\multicolumn{5}{c}{\textbf{Selected feature analysis}}\\
     \multicolumn{5}{c}{\textbf{Morpheme analysis}} & \textbf{NDW} & \textbf{TTR} & \textbf{CTTR} & \textbf{NNL\_Den} & \textbf{EFL\_Den} \\
    \cmidrule(r){1-5} \cmidrule(l){6-10}
    \makecell*{\textbf{\underline{나\tiny{/NP}\normalsize{+는}\tiny{/JX}}} \\ \textbf{\underline{\textit{Na-neun}}}} & \makecell*{하늘\tiny{/NNG}\normalsize{+을}\tiny{/JKO} \\ \textit{haneur-eul}} & \makecell*{\textbf{\underline{날\tiny{/VV}\normalsize{+는}\tiny{/ETM}}} \\ \textbf{\underline{\textit{Nal-neun}}}} & \makecell*{나비\tiny{/NNG}\normalsize{+를}\tiny{/JKO} \\ \textit{nabi-reul}} & \makecell*{보\tiny{/VV}\normalsize{+았}\tiny{/EP}\normalsize{+다}\tiny{/EF} \\ \textit{bo-at-da}} & \(10\) & \(\frac{10}{11}\approx 0.91\) & \(\frac{10}{\sqrt{22}}\approx 2.13\) & \(\frac{3}{11}\approx 0.27\) & \(\frac{3}{6}\approx 0.50\)  \\
    \cmidrule(r){1-5} \cmidrule(l){6-10}
    \makecell*{\textbf{\underline{나\tiny{/NP}\normalsize{+는}\tiny{/JX}}} \\ \textbf{\underline{\textit{Na-neun}}}} & \makecell*{하늘\tiny{/NNG}\normalsize{+을}\tiny{/JKO} \\ \textit{haneur-eul}} & \ash{\makecell*{\textbf{\underline{나\tiny{/NP}\normalsize{+는}\tiny{/JX}}} \\ \textbf{\underline{\textit{Na-neun}}}}} & \makecell*{나비\tiny{/NNG}\normalsize{+를}\tiny{/JKO} \\ \textit{nabi-reul}} & \makecell*{보\tiny{/VV}\normalsize{+았}\tiny{/EP}\normalsize{+다}\tiny{/EF} \\ \textit{bo-at-da}} & \ash{\(9\)} & \ash{\(\frac{9}{11}\approx 0.82\)} & \ash{\(\frac{9}{\sqrt{22}}\approx 1.92\)} & \ash{\(\frac{4}{11}\approx 0.36\)} & \ash{\(\frac{2}{6}\approx 0.33\)} \\

    \bottomrule
\end{tabular}
}
\label{tb:error_prop}
\end{table*}
%===================================================================

\section{Appendices}
\subsection{Importance of Error Propagation}
This section describes the importance of Korean morpheme analysis.
Table \ref{tb:error_prop} illustrates how morpheme analysis results should differ, `나\tiny{/NP}\normalsize{+는}\tiny{/JX}\normalsize{ (\textit{Na-Neun})' and `날}\tiny{/VV}\normalsize{+는}\tiny{/ETM}\normalsize{ (\textit{Nal-Neun})'}, even for the same type of wordpiece `나는 (\textit{Naneun})'. 
This example highlights the difficulties in achieving accurate morpheme analysis. 
Moreover, as shown at the bottom of Table \ref{tb:error_prop}, errors can distort the values of some features, reducing the reliability of feature analysis and writing evaluation.

\subsection{Morpheme Description}
See Table \ref{tb:postag}.
%===================================================================
\begin{table*}[tbh!]
\centering
\caption{\textbf{Information of POS tag.} }
% Roman expressions in Korean are denoted using \textit{italic}.}
\resizebox{0.7\textwidth}{!}{%
% \begin{threeparttable}
\setlength\tabcolsep{9.3pt}
\begin{tabular}{cllc}
    \toprule
    \textbf{Category} & \textbf{Sub-category} & \textbf{Morpheme} & \textbf{POS tag} \\ 
    \midrule
    \multirow{5}{*}{\textbf{\underline{N}oun}} & \multirow{3}{*}{\textbf{N}oun} & \textbf{G}enaral noun & NNG \\
     &  & \textbf{P}roper noun & NNP \\
     &  & \textbf{B}ound noun & NNB \\
     \cmidrule(l){2-4} 
     & \textbf{P}ronoun && NP \\
     & Nume\textbf{r}al && NR \\
    \midrule
    \multirow{5}{*}{\textbf{\underline{V}erb}} & \textbf{V}erb && VV \\
     & \textbf{A}djective && VA \\
     & Au\textbf{x}iliary verb && VX \\
     \cmidrule(l){2-4} 
     & \multirow{2}{*}{\textbf{C}opula} & \textbf{P}ositive copula & VCP \\
     &  & \textbf{N}egative copula & VCN \\
    \midrule
    \multirow{5}{*}{\textbf{\underline{M}odifier}} & \multirow{3}{*}{Adno\textbf{m}inal} & \textbf{A}dnominal modifier & MMA \\
     &  & \textbf{D}emonstrative modifier & MMD \\
     &  & \textbf{N}umeral modifier & MMN \\
     \cmidrule(l){2-4} 
     & \multirow{2}{*}{\textbf{A}dverb} & \textbf{G}eneral adverb & MAG \\
     &  & Con\textbf{j}unction adverb & MAJ \\
    \midrule
    \textbf{\underline{I}nterje\underline{c}tion} & Interjection && IC \\
    \midrule
    \multirow{10}{*}{\makecell*{\textbf{Postposion} \\ \textbf{(\textit{\underline{J}osa)}}}} & \multirow{7}{*}{
    \makecell*{Case marker \\ (\textit{\textbf{K}yeok-josa})}} 
     & \textbf{S}ubject case marker & JKS \\
     &  & \textbf{C}omplement case marker & JKC \\
     &  & Adnominal (\textit{\textbf{G}wanhyeong-kyeok}) case marker & JKG \\
     &  & \textbf{O}bject case marker & JKO \\
     &  & Adverbial (\textit{\textbf{B}usa-kyeok}) case marker & JKB \\
     &  & \textbf{V}ocative case marker & JKV \\
     &  & \textbf{Q}uotative case marker & JKQ \\
     \cmidrule(l){2-4} 
     & Au\textbf{x}iliary && JX \\
     & \textbf{C}onjunctive && JC \\
    \midrule
    \multirow{5}{*}{\textbf{\underline{E}nding}} & \multicolumn{2}{l}{\textbf{P}refinal ending} & EP \\
     & \multicolumn{2}{l}{\textbf{F}inal ending} & EF \\
     & \multicolumn{2}{l}{\textbf{C}onnective ending}& EC \\
     \cmidrule(l){2-4}
     & \multirow{2}{*}{\textbf{T}ransformative} & \textbf{N}oun ending & ETN \\
     & & Adno\textbf{m}inal ending & ETM \\
    \midrule
    \multirow{5}{*}{\textbf{Affi\underline{x}}} & \textbf{P}refix & \textbf{N}oun prefix & XPN \\
     \cmidrule(l){2-4} 
     & \multirow{3}{*}{\textbf{S}uffix} & \textbf{N}oun suffix & XSN \\
     &  & \textbf{V}erb suffix & XSV \\
     &  & \textbf{A}djective suffix & XSA \\
     \cmidrule(l){2-4} 
     & \textbf{R}oot && XR \\
    \midrule
    \multirow{9}{*}{\textbf{\underline{S}ign}} & \multirow{6}{*}{Symbol} & \textbf{F}inal symbol (. ? !) & SF \\
     && \textbf{P}ause symbol (, : ; /) & SP \\
     && Quotation marks (``" `'), bracket ({[}{]} \{\} ()), dash (-) & SS \\
     && \textbf{E}llipsis (…) & SE \\
     && Swung dash ($\sim$) & SO \\
     && Etc. & SW \\
     \cmidrule(l){2-4} 
     & Foreign \textbf{l}anguage && SL \\
     & \multicolumn{2}{l}{Chinese character (\textit{\textbf{H}anja)}} & SH \\
     & \textbf{N}umber && SN \\ 
     \bottomrule
     %\cmidrule(l){2-4} 
\end{tabular}
}
\label{tb:postag}
\end{table*}
%===================================================================

\subsection{Lexical Feature Description}
See Table \ref{tb:postag}.

\subsection{Rubric Description}
See Table \ref{tb:postag}.

\subsection{More Korean Writing Evaluation Results}
See Table \ref{tb:postag}.

\subsection{More Visualization Results}
See Table \ref{tb:postag}.
